# Supplementary material for: Acceleration and radiation: Classical and quantum aspects
Source: arXiv:2406.17980 source file (2024-06-25)
Supplement: Supplementary file 1 [file geometry.tex]

% !TEX encoding = UTF-8

% Class of the document, we use the KOMA article
\documentclass[DIV=17]{scrartcl}

%%%%%%%%%%%%%%%%%%%%%%%%%%%%%%%%%%%%%%%%%%%%%%%%%%%%%%%%%%%%%%%%%%%%%%%%%%%%%%%%
%%%%% PACKAGES and MACROS
%%%%%%%%%%%%%%%%%%%%%%%%%%%%%%%%%%%%%%%%%%%%%%%%%%%%%%%%%%%%%%%%%%%%%%%%%%%%%%%%

\usepackage[utf8]{inputenc} % input encoding 
\usepackage[english]{babel} % language
\usepackage{stix,inconsolata} %fonts
\usepackage[scale=0.94]{tgheros}
\usepackage{amsmath,physics,tikz,csquotes,amsfonts} % add usability and math support
\usepackage[style=abnt,justify,indent,language=english]{biblatex} % bibliography
\usepackage[T1]{fontenc} % output encoding
\usepackage[colorlinks,allcolors=blue!40!black]{hyperref} % clickable links

% bibliography files
\addbibresource{../acceleration_and_radiation.bib}

%%%%%%%%%%%%%%%%%%%%%%%%%%%%%%%%%%%%%%%%%%%%%%%%%%%%%%%%%%%%%%%%%%%%%%%%%%%%%%%%
%%%%% METADATA FOR THE DOCUMENT
%%%%%%%%%%%%%%%%%%%%%%%%%%%%%%%%%%%%%%%%%%%%%%%%%%%%%%%%%%%%%%%%%%%%%%%%%%%%%%%%

\title{The geometry of spacetime}
\author{Felipe Ignacio Portales Oliva}
\date{Started: 7th July 2021; version of: \today}

%%%%%%%%%%%%%%%%%%%%%%%%%%%%%%%%%%%%%%%%%%%%%%%%%%%%%%%%%%%%%%%%%%%%%%%%%%%%%%%%
%%%%% THE DOCUMENT ITSELF
%%%%%%%%%%%%%%%%%%%%%%%%%%%%%%%%%%%%%%%%%%%%%%%%%%%%%%%%%%%%%%%%%%%%%%%%%%%%%%%%
\begin{document}
	
\maketitle

In this chapter we aim to briefly present the geometric quantities that arise in the study of Einstein's general relativity \cite{Einstein1915} for the sake of
consistency and to avoid confusing the reader with our notation, as there are many of them used in different parts of the literature (the choice of index
locations and names is up to each author). 

\section{Basic notions}

A \( d \)-dimensional Haussdorf manifold \( M \) is a set of \emph{points} such that the collection of subsets of \( M \), each denoted by \( U_\alpha \) (\(
\alpha \) is a general index), which are known as open sets, satisfy 
\begin{equation}
    M = \bigcup_{\forall \alpha} U_\alpha,
    \label{eq:union-of-open-sets}
\end{equation}
and for each of the open sets there is a smooth bijective mapping 
\begin{equation}
    x\!:\ U_\alpha \longrightarrow x(U_\alpha)\subseteq\mathbb{R}^d,
    \label{eq:coordinate definition}
\end{equation}
called the \emph{local coordinate patch}, such that 
\begin{enumerate}
    \item for two opens \( U_\alpha \) and \( U_\beta \), each with its own coordinate patch \( x \) and \( y \) respectively, if \( U_\alpha \cap U_\beta \neq \emptyset \) the isomorphisms 
    \begin{subequations}
        \begin{gather}
            x \circ y^{-1} \! : y(U_\alpha \cap U_\beta) \subseteq\mathbb{R}^d \longrightarrow x(U_\alpha \cap U_\beta) \subseteq\mathbb{R}^d,
            \\
            y \circ x^{-1} \! : x(U_\alpha \cap U_\beta) \subseteq\mathbb{R}^d \longrightarrow y(U_\alpha \cap U_\beta) \subseteq\mathbb{R}^d,
        \end{gather}
    \end{subequations}
    are well defined (these are known as the \emph{coordinate transformations} or \emph{diffeomorphisms}); and 
    \item for two different points \( P, Q \in M \) there exist two open sets \( U_P, U_Q \subset M \) with \( P\in U_P \) and \( Q \in U_Q \) such that \( U_P
    \cap U_Q = \emptyset \) (the Haussdorf condition).
\end{enumerate}
Geometrical quantities of interest (scalar, vectors, etc.) are generally \emph{covariant} under diffeomorphisms, this is, they follow a certain transformation
rules under coordinate changes depending on the object. 

Going on forward (and in the entirety of this thesis), we will deal with 4-dimensional spacetime. We will also use two distinct coordinate patches \( x \) and
\( x' \) defined in a single open \( U \) for the following of this discussion, and use the latin indices \( a,b,c,\ldots \) to label each \emph{component} of
the geometrical objects; each index runs from 0 to 3 and we assume Einstein's summation convention is used.  

The simplest of the transformation rules for quantities we are interested in, are the ones for \emph{scalars}, generally defined by a mapping like
\begin{equation}
    \phi \! : U \subseteq M \longrightarrow \mathbb{R},
    \label{eq:definition-scalar}
\end{equation}
as these assign a single value to each point in the open \( U \), this value must be the same independently of the coordinates used to describe the point in the
manifold, i.e., for \( P \in U \subseteq M \) we have 
\begin{equation}
    \phi (P) 
        = \phi \boldsymbol{(} x(P) \boldsymbol{)} 
        = \phi \boldsymbol{(} x'(P) \boldsymbol{)},
    \label{eq:}
\end{equation}

\printbibliography
\end{document}
